# Supplementary material for: DISCOVER: A Physics-Informed, GPU-Accelerated Symbolic Regression Framework
Source: arXiv:2602.06986 ancillary file (2026-01-27)
Supplement: Supplementary file 1 [file Supplementary_Material.pdf]

# DISCOVER

A Supplementary Material / Mathematical Guide

January 27, 2026

# 1 The Core Problem: $L_0$-Regularized Regression

All search methods in DISCOVER are designed to find an approximate or exact solution to the same fundamental problem. Given a large set of $M$ candidate symbolic features $\Phi = \{\Phi_1, \Phi_2, \ldots, \Phi_M\}$ and a target property vector $\mathbf{y}$, the goal is to find a linear model with at most $D$ features that minimizes the prediction error. This is the $L_0$-norm regularized least-squares problem:

$$\min_{\beta} \|\mathbf{y} - \Phi\beta\|_2^2 \quad \text{subject to} \quad \|\beta\|_0 \leq D \tag{1}$$

where $\|\beta\|_0$ counts the number of nonzero elements in the coefficient vector $\beta$. This problem is NP-hard, necessitating the use of various exact heuristic, approximate, or specialized algorithms.

# 2 Search Algorithms (The Sparsifying Operator)

The following methods are implemented in `search.py` to select the optimal subset of $D$ features from the screened candidates.

## 2.1 Brute-Force Search (`_find_best_models_brute_force`)

### 2.1.1 Methodology

This is the most straightforward and exhaustive approach. It systematically evaluates every possible combination of $D$ features from the pool of $M$ candidates.

1. For a given dimension $D$, generate all $\binom{M}{D}$ unique combinations of features.

2. For each combination, form a feature matrix $X_D$.

3. Fit an Ordinary Least Squares (OLS) regression model to find the coefficients $\beta$.

$$\beta = X_D^{\dagger}\mathbf{y} \quad \text{(pseudo-inverse in case } X_D \text{ is rank-deficient)}$$

4. Calculate the error of this model, typically the Root Mean Squared Error (RMSE).

$$\text{RMSE} = \sqrt{\frac{1}{n}\sum_{i=1}^{n}(y_i - \hat{y}_i)^2} = \sqrt{\frac{1}{n}\|\mathbf{y} - X_D\beta\|_2^2}$$

5. The combination that yields the minimum RMSE is selected as the best model for dimension $D$.

### 2.1.2 Application in Symbolic Regression

This method guarantees finding the globally optimal set of $D$ symbolic features from the selected screened pool. However, its computational cost, $O(\binom{M}{D})$, makes it practical only for very small $M$ and $D$.

## 2.2 Greedy Search (`_find_best_models_greedy`)

### 2.2.1 Methodology

This is a forward selection algorithm that builds the model one feature at a time. It is computationally efficient, but may not find the global optimum.

1. **Dimension 1:** Find the single best feature $\Phi_1^*$ by fitting $M$ separate 1D models. The feature with the lowest error is selected.

$$\Phi_1^* = \underset{\Phi_j \in \Phi}{\operatorname{argmin}} \left( \min_{\beta_0, \beta_j} \|\mathbf{y} - (\beta_0 + \beta_j \Phi_j)\|_2^2 \right)$$

2. **Dimension 2:** Keep $\Phi_1^*$ fixed. Search through all remaining $M-1$ features to find the second feature $\Phi_2^*$ that, when combined with $\Phi_1^*$, yields the best 2D model.

$$\Phi_2^* = \underset{\Phi_j \in \Phi \setminus \{\Phi_1^*\}}{\operatorname{argmin}} \left( \min_{\beta_0, \beta_1, \beta_j} \|\mathbf{y} - (\beta_0 + \beta_1 \Phi_1^* + \beta_j \Phi_j)\|_2^2 \right)$$

3. **Dimension D:** Continue this process, adding one feature at each step that provides the greatest improvement to the existing model, until a $D$-dimensional model is constructed.

### 2.2.2 Application in Symbolic Regression

The greedy search quickly identifies a good, but not necessarily optimal, combination of symbolic features. In each step, it selects the symbolic expression that best explains the variance *not already explained* by the previously selected features.

## 2.3 Orthogonal Matching Pursuit (OMP) (`_find_best_models_omp`)

### 2.3.1 Methodology

OMP is a more robust version of the greedy algorithm. Instead of just adding the next best feature, it recalculates the coefficients for all selected features at each step.

1. Initialize the residual $\mathbf{r}_0 = \mathbf{y}$ and the selected feature set $\mathcal{S}_0 = \emptyset$.

2. For $k = 1, \ldots, D$:

   (a) Find the feature $\Phi_k^*$ from the remaining pool that is most correlated with the current residual $\mathbf{r}_{k-1}$.

$$\Phi_k^* = \underset{\Phi_j \notin \mathcal{S}_{k-1}}{\operatorname{argmax}} |\langle \mathbf{r}_{k-1}, \Phi_j \rangle|$$

   (b) Add the selected feature to the active set: $\mathcal{S}_k = \mathcal{S}_{k-1} \cup \{\Phi_k^*\}$.

   (c) Solve a least-squares problem to find the new coefficients $\beta_k$ using all features currently in the active set $\mathcal{S}_k$.

$$\beta_k = \Phi_{\mathcal{S}_k}^{\dagger} \mathbf{y} \quad \text{(least-squares solution / pseudo-inverse)}$$

   (d) Update the residual for the next iteration.

$$\mathbf{r}_k = \mathbf{y} - \Phi_{\mathcal{S}_k} \beta_k$$

### 2.3.2 Application in Symbolic Regression

OMP provides a more stable path to a solution than a simple greedy search. By re-fitting the entire model at each step, it better accounts for correlations between the selected symbolic features, often leading to a more physically meaningful final equation.

## 2.4 SISSO++ (Breadth-First QR Search) (`_find_best_models_sisso_pp`)

### 2.4.1 Methodology

This is a highly efficient breadth-first search algorithm that avoids the combinatorial explosion of brute-force by using linear algebra updates. It keeps a "beam" of the best-performing models at each dimension.

1. **Dimension 1:** Evaluate all 1D models and retain the top $N_{\text{beam}}$ models with the lowest RSS.

2. **Dimension 2:** For each of the $N_{\text{beam}}$ models from D=1, try adding every other available feature.

3. **The QR Update:** The key to its efficiency is using QR decomposition. If we have the decomposition for a feature set $X_D = Q_D R_D$, the RSS is easily calculated:

$$\text{RSS}_D = \|\mathbf{y}\|_2^2 - \|Q_D^T \mathbf{y}\|_2^2$$

   To find the RSS for a new model with an added feature $\mathbf{x}_{\text{new}}$, we don't refit. Instead, we compute the component of $\mathbf{x}_{\text{new}}$ orthogonal to the space spanned by $Q_D$:

$$\mathbf{w}_{\text{new}} = \mathbf{x}_{\text{new}} - Q_D Q_D^T \mathbf{x}_{\text{new}}$$

   The reduction in RSS is then calculated directly:

$$\Delta\text{RSS} = \frac{(\mathbf{r}_D^T \mathbf{w}_{\text{new}})^2}{\|\mathbf{w}_{\text{new}}\|_2^2}$$

   where $\mathbf{r}_D = \mathbf{y} - Q_D Q_D^T \mathbf{y}$ is the residual.

4. A new beam of the top $N_{\text{beam}}$ 2D models is created, and the process repeats for $D = 3, \ldots, D_{\text{max}}$.

### 2.4.2 Application in Symbolic Regression

SISSO++ explores a much wider range of feature combinations than a simple greedy search without incurring the cost of brute-force. It is highly effective at finding high-quality, low-dimensional symbolic models that might be missed by a purely sequential greedy approach.

## 2.5 Random Mutation Hill Climbing (RMHC) & Simulated Annealing (SA)

### 2.5.1 Methodology

These are stochastic heuristic search algorithms that explore the solution space by making random changes to a candidate model.

- **RMHC (`_find_best_models_rmhc`):**

  1. Start with a good initial $D$-dimensional model (e.g., from a greedy search).
  2. In each iteration, randomly swap one feature in the current model with one feature from the outside pool.

3. If the new model has a lower error (is "uphill"), accept the change.
4. If the new model is worse, reject the change and keep the old model.
5. Repeat for many iterations. Multiple restarts from the best-so-far solution help avoid local optima.

- **SA (`_find_best_models_sa`):** SA is similar to RMHC, but with a crucial difference: it can accept "downhill" moves (worse solutions) to escape local optima. The probability of accepting a worse solution with error increase $\Delta E$ is given by the Metropolis criterion:

$$P(\text{accept}) = e^{-\frac{\Delta E}{T}}$$

where $T$ is a "temperature" parameter that starts high (allowing many bad moves) and is gradually decreased (the "annealing schedule"), making the search converge towards a good solution.

#### 2.5.2 Application in Symbolic Regression

These methods are excellent for refining a model found by a faster method like a greedy search. They can escape the local optima that greedy methods are prone to, potentially swapping out a feature for another that, while worse on its own, enables a much better overall model when combined with the other $D-1$ features.

### 2.6 Mixed-Integer Quadratic Programming (MIQP) (`_find_best_models_miqp`)

#### 2.6.1 Methodology

This method provides a mathematically rigorous, exact solution to the $L_0$ problem. It recasts the problem into a format that can be solved by specialized solvers like Gurobi.

1. **Variables:** Define two sets of variables:
   - Continuous variables $\beta_j$ for the coefficients.
   - Binary variables $z_j \in \{0,1\}$, where $z_j = 1$ if feature $\Phi_j$ is included in the model, and 0 otherwise.
2. **Objective Function:** Minimize the RSS, which is a quadratic function of $\beta$.

$$\min_{\beta,\mathbf{z}} \quad (\mathbf{y}-\Phi\beta)^T(\mathbf{y}-\Phi\beta) \quad \equiv \quad \min_{\beta,\mathbf{z}} \quad \beta^T(\Phi^T\Phi)\beta - 2(\mathbf{y}^T\Phi)\beta + \mathbf{y}^T\mathbf{y}$$

3. **Constraints:**
   - The **Cardinality Constraint** directly enforces the $L_0$ norm:

$$\sum_{j=1}^{M} z_j = D$$

   - The **Big-M Constraints** link the binary and continuous variables. They ensure that if a feature is not selected ($z_j = 0$), its coefficient must also be zero ($\beta_j = 0$).

$$-M \cdot z_j \le \beta_j \le M \cdot z_j \quad \text{for } j = 1, \ldots, M$$

   where $M$ is a sufficiently large constant (an upper bound on any possible coefficient value).

### 2.6.2 Application in Symbolic Regression

When applicable (for regression with $L_2$ loss) and computationally feasible, MIQP is the gold standard. It guarantees that the selected combination of $D$ symbolic features is the provably optimal one from the entire candidate pool, leaving no doubt that a better linear combination of $D$ features exists.

## 2.7 Geometric Greedy Search (`_find_best_models_ch_greedy`)

### 2.7.1 Methodology

This is a specialized greedy search for the `ch_classification` task. The scoring function is not RMSE but a geometric measure of class separability.

1. At each dimension $D$, the goal is to add a new feature that minimizes the overlap between the convex hulls of the different classes in the $D$-dimensional descriptor space.

2. The overlap is estimated using **Monte Carlo integration**:

   (a) A large number of random points are sampled within the bounding box of the data.

   (b) For each point, determine how many class hulls it falls inside.

   (c) The overlap score is the fraction of points inside any hull that are also inside more than one hull.

   $$\text{Overlap Fraction} = \frac{\text{Points in } \geq 2 \text{ hulls}}{\text{Points in } \geq 1 \text{ hull}}$$

3. The search proceeds greedily, selecting the feature at each step that results in the lowest overlap fraction.

### 2.7.2 Application in Symbolic Regression

This method finds a set of symbolic features that transform the original data into a new space where the different classes are maximally separable by geometric boundaries (convex hulls). The resulting "formula" is not a single equation for a property, but a set of coordinate transformations (the descriptors) that define this optimal classification space.

# 3 Post-Search: Non-Linear Refinement (`_refine_model_with_nlopt`)

After a linear model has been identified by one of the search methods, this optional step can refine it by introducing non-linear parameters.

- **Methodology:** It takes a discovered linear model, such as $y \approx \beta_0 + \beta_1\Phi_1 + \beta_2\Phi_2$, and tests if replacing a descriptor $\Phi_i$ with a parameterized version, like $e^{-p\Phi_i}$ or $\Phi_i^p$, can improve the fit.

- It uses a numerical optimization algorithm (L-BFGS-B) to simultaneously find the optimal values for the linear coefficients ($\beta_i$) and the new non-linear parameters ($p$). The objective function remains the RMSE.

- **Application in Symbolic Regression:** This allows DISCOVER to find even more complex and accurate formulas that are not purely linear combinations of the base descriptors, such as discovering optimal exponents or decay constants within the final equation.

# DISCOVER User Guide: Configuration and Execution

A Scientific Discovery Tool

## A Configuration with `config.json`

The DISCOVER workflow is controlled by a single JSON configuration file. This file allows users to define the dataset, specify the feature generation grammar, control the search and validation strategies, and set computational parameters. Below is a detailed explanation of each parameter. Additional details can be found: https://u-gajera.github.io/discover/

### 1. Data & I/O Settings

This section defines the input data and output locations.

`data_file` (string): Path to the input data file. The current implementation supports CSV format.

`property_key` (string): The column name in the data file corresponding to the target property (the dependent variable, $y$). For multi-task regression, this can be a list of column names.

`non_feature_cols` (list of strings): A list of columns to exclude from being used as primary features. This is useful for identifiers or metadata columns.

`workdir` (string): The name of the directory where all output files, models, and plots will be saved. If the directory exists, the user will be prompted before overwriting.

`save_feature_space` (boolean): If true, the entire generated feature space (after iterative screening) is saved to a compressed CSV file (`feature_space.csv.gz`) in the workdir. This can be useful for debugging or external analysis but may consume significant disk space.

`use_cache` (boolean): If true, enables caching for feature generation. This dramatically speeds up repeated runs with the same feature generation settings by storing intermediate results in the workdir.

### 2. Feature-Space Construction

This section governs the symbolic feature engineering process.

`depth` (integer): The maximum depth of the operator tree for feature generation. A depth of 1 applies operators to primary features. A depth of 2 applies operators to the results of depth 1, and so on. This is the primary control for the complexity of generated features.

`op_rules` (list of dicts): Defines the set of mathematical operators used to build new features. The simplest form is a list of operator names, e.g., `[{"op": "add"}, {"op": "sub"}]`. Built-in operators include:

- **Binary**: `add, sub, mul, div, abs_diff, harmonic_mean`.
- **Unary**: `inv, abs, sq` (square), `cb` (cube), `sqrt, cbrt, log, exp, exp-` (exp(-x)), `sin, cos, sign`.

`parametric_ops` (list of strings): A list of parametric operators to be used in a final non-linear refinement step after the main search. Current options include `'exp-'` (e.g., $e^{-p\cdot x}$) and `'pow'` (e.g., $x^p$), where $p$ is a free parameter optimized by the algorithm. This is only active for regression tasks.

`primary_units` (dict): A dictionary mapping primary feature names (column headers) to their physical units. This enables `pint`-based dimensionality checking, ensuring that only dimensionally valid operations (e.g., addition of same-unit quantities, logarithm of dimensionless quantities) are performed. This is a critical feature for scientific applications.

`min_abs_feat_val`, `max_abs_feat_val` (float): Minimum and maximum absolute values allowed for any generated feature. This helps prevent numerical instability (underflow/overflow).

## 3. Search & Selection Strategy

This section defines how the best descriptor model is identified from the vast feature space.

`max_D` (integer): The maximum dimension (number of terms) of the final descriptor to search for. The algorithm will find the best 1-D, 2-D, ..., up to `max_D`-dimensional models.

`sis_sizes` (list of integers): In the iterative framework, only the first element is used. It specifies the number of top features to retain after Sure Independence Screening (SIS) at each `depth` of feature generation.

`search_strategy` (string): The algorithm used to find the best D-dimensional descriptor from the screened feature space. Options: `'greedy'`, `'brute_force'`, `'omp'`, `'sisso++'`, `'rmhc'`, `'sa'`, `'miqp'`. A detailed explanation of each strategy is provided in Section A.6.

`max_feat_cross_correlation` (float): A threshold (0.0 to 1.0) used to prune the feature space by removing highly correlated features before the main search begins. A value of 0.95 means that from any cluster of features correlated ¿0.95, only one is kept.

## 4. Model Construction & Validation

This section controls the final model fitting and selection process.

`task_type` (string): Specifies the type of machine learning problem. This determines the model and scoring function. Options: `'regression'`, `'multitask'`, `'classification_svm'`, `'classification_logreg'`, `'ch_classification'`.

`selection_method` (string): The method used to select the best dimension (`D`) from the models found.

- `'cv'`: K-Fold Cross-validation.
- `'bootstrap'`: Bootstrap with out-of-bag (OOB) error estimation.
- `'aic'`/`'bic'`: Akaike/Bayesian Information Criterion (for regression only).

`cv` (integer): The number of folds for cross-validation. Set to -1 for Leave-One-Out CV (LOOCV).

`fix_intercept` (boolean): If true, the linear model is fitted without an intercept term ($\beta_0 = 0$).

## 5. Computational Settings

`n_jobs` (integer): The number of CPU cores to use for parallelized tasks. Set to -1 to use all available cores.

`device` (string): The computational device for accelerated calculations. Options: `'cpu'`, `'cuda'` (for NVIDIA GPUs, requires `cupy`), `'mps'` (for Apple Silicon GPUs, requires `pytorch`). GPU acceleration is available for feature generation and certain search/scoring functions.

`random_state` (integer): A seed for the random number generator to ensure reproducibility of results.

## 6. Advanced Feature Selection and Search Strategies

DISCOVER includes several advanced methods for both screening candidate features and searching for the final descriptor. These methods offer trade-offs between computational cost, robustness, and the ability to capture complex relationships.

### Leave-One-Out Cross-Validation (LOOCV)

**Purpose:** LOOCV is an exhaustive form of cross-validation where the number of folds is equal to the number of data points. For a dataset of size $N$, it trains $N$ separate models, each on $N-1$ points, and validates on the single held-out point.

**When to Use:** It is highly recommended for **small datasets** (e.g., $N < 100$) where K-Fold CV might yield volatile results due to the small size of the validation sets. It provides a nearly unbiased estimate of model performance but is computationally very expensive for large datasets.

**Configuration:** To enable LOOCV, set the `cv` parameter to `-1`.

```
"selection_method": "cv",
"cv": -1

```

**Compatibility:** Can be used with any `task_type`.

### Decision Tree Feature Screening

**Purpose:** This method replaces the default correlation-based screening (SIS) with a more sophisticated approach. It scores features based on a combination of their importance in a trained decision tree model (the likelihood) and their symbolic complexity (the prior). The final score favors features that are both predictive and simple.

**When to Use:** Use when you suspect that the relationship between features and the target is highly **non-linear or involves complex interactions**. Standard correlation might miss features that are only important in specific regimes. This method is slower than correlation-based screening but can lead to a higher-quality feature space.

**Configuration:** Set the `sis_method` parameter.

```
"sis_method": "decision_tree"

```

**Compatibility:** Works for both `regression` and `classification` tasks. For multi-task regression, it treats the problem as a standard multi-output regression task. It is a CPU-only feature.

### Search Strategy: Greedy ('greedy')

**Purpose:** The default search strategy. This is a forward-selection algorithm that builds the descriptor one feature at a time. In the first step, it selects the single best feature. In the second step, it finds the next feature that, when added to the first, best explains the *residual* (the remaining error). It continues this process until the desired dimension is reached.

**When to Use:** This is the fastest search algorithm and serves as an excellent baseline. It is a good first choice for exploring a new problem, but it can be susceptible to finding local optima.

**Compatibility:** Can be used with any `task_type`.

### Search Strategy: Brute-Force ('brute_force')

**Purpose:** This method exhaustively evaluates every possible combination of features for a given dimension. It guarantees that the returned model is the true optimum for that dimension from the given feature space.

**When to Use:** Use when the number of candidate features and the maximum dimension are both small, and you want to be certain you have found the best possible linear model. The number of combinations grows factorially, so this becomes computationally infeasible very quickly.

**Compatibility:** Can be used with any `task_type`.

**Search Strategy: Orthogonal Matching Pursuit (`'omp'`)**

**Purpose:** OMP is a greedy algorithm that improves upon the standard greedy search. At each step, it selects the feature that is most correlated with the *current residual* of the model. After adding the new feature, it refits the model on the *entire set* of selected features using ordinary least squares. This re-fitting step makes it more robust than a simple greedy search.

**When to Use:** OMP is a fast, robust, and reliable choice for most regression problems. It provides a good balance between speed and quality of the solution, often outperforming the standard greedy search.

**Compatibility:** This method is designed for `regression` and `multitask` regression tasks only.

**Search Strategy: SISSO++ (`'sisso++'`)**

**Purpose:** This is a highly efficient breadth-first search algorithm. It intelligently explores the search space by building up descriptors dimension by dimension, keeping a "beam" of the best candidates at each level. Its speed comes from using QR decomposition updates to efficiently calculate the residual sum of squares without refitting the model from scratch for each new combination.

**When to Use:** SISSO++ is an excellent choice for large feature spaces where brute-force is infeasible. It is often much faster than other search methods for higher dimensions ($D > 2$) and can be GPU-accelerated for regression tasks.

**Configuration:**
```
"search_strategy": "sisso++",
"beam_width_decay": 1.0

```

- `beam_width_decay`: A factor ($\leq 1.0$) to shrink the search beam at each dimension. A value of 1.0 keeps the beam size constant, while a value like 0.8 speeds up the search for higher dimensions by focusing only on the most promising candidates.

**Compatibility:** Can be used with any `task_type`. For classification and multitask problems, it uses an Ordinary Least Squares proxy for the search phase, with a final refit using the correct model.

**Search Strategy: Random Mutation Hill Climbing (`'rmhc'`)**

**Purpose:** RMHC is a metaheuristic search algorithm that refines an existing solution. It starts with a good "seed" model (found via a fast greedy search) and then iteratively tries to improve it by making small, random changes ("mutations"). A mutation consists of swapping one feature in the current descriptor with a random feature from the wider pool. If the change improves the model's score, it is accepted.

**When to Use:** RMHC is an excellent choice when you want a more thorough search than a simple greedy algorithm but cannot afford the computational cost of brute-force. It is very effective at finding small improvements and escaping the local optima that can trap a greedy search.

**Configuration:**
```
"search_strategy": "rmhc",
"rmhc_iterations": 200,
"rmhc_restarts": 5

```

- `rmhc_iterations`: The number of mutations to attempt for each restart.
- `rmhc_restarts`: The number of times the hill-climbing process is restarted from the best-known solution. Multiple restarts help ensure the search is not permanently stuck on a suboptimal peak.

**Compatibility:** Can be used with any `task_type`.

**Search Strategy: Simulated Annealing (`'sa'`)**

**Purpose:** SA is a powerful global optimization technique inspired by annealing in metallurgy. It starts by exploring the feature space broadly (high "temperature") and gradually narrows its search to promising regions (low "temperature"). Unlike hill climbing, SA can accept a worse solution with a certain probability, allowing it to escape local optima and find a potentially better global optimum.

**When to Use:** SA is one of the most robust search strategies. Use it when the feature space is likely rugged with many local minima and you need a high-confidence global search without resorting to brute-force. It is generally slower than RMHC but more likely to find the global optimum.

**Configuration:**
```
"search_strategy": "sa",
"sa_initial_temp": 1.0,
"sa_final_temp": 1e-4,
"sa_cooling_rate": 0.99,
"sa_acceptance_rule": "metropolis"

```

- `sa_initial_temp`: The starting temperature. Higher values encourage more exploration.
- `sa_final_temp`: The temperature at which the search terminates.
- `sa_cooling_rate`: The factor by which the temperature is multiplied at each step. Values closer to 1.0 mean slower, more thorough cooling.
- `sa_acceptance_rule`: The criterion for accepting a worse move. `'metropolis'` uses $P = e^{-\Delta E/T}$, while `'glauber'` uses $P = 1/(1 + e^{\Delta E/T})$. Metropolis is more common.

**Compatibility:** Can be used with any `task_type`.

**Search Strategy: Mixed-Integer Quadratic Programming (`'miqp'`)**

**Purpose:** This strategy formulates the descriptor selection problem as a formal mathematical optimization problem. It finds the **provably optimal** set of features that minimizes the L0-norm (i.e., the number of non-zero coefficients) for a given descriptor dimension.

**When to Use:** Use MIQP when you require mathematical proof of optimality for the final model and the feature space is of a manageable size (typically a few hundred features). It is computationally intensive and relies on an external solver.

**Configuration:**
```
"search_strategy": "miqp"

```

**Compatibility:** This method is only available for `regression` tasks with an `'l2'` loss. It requires the `gurobipy` Python package and a valid Gurobi license.

**Example:** `config.json`

```
{
  // ==================================================================
  //                         1. DATA & I/O SETTINGS
  // ==================================================================
  "data_file":                 "Sample_Dataset.csv",
  "property_key":              "Target_U (eV)",
  "non_feature_cols":          ["material_id"],
  "workdir":                   "discover_output",
  "save_feature_space":        false,

  // ==================================================================
  //                    2. FEATURE-SPACE CONSTRUCTION
  // ==================================================================
  "depth":                     2,
  "op_rules": [
    {"op": "add"}, {"op": "sub"}, {"op": "mul"}, {"op": "div"},
    {"op": "inv"}, {"op": "abs"}, {"op": "sq"}, {"op": "cb"},
    {"op": "sqrt"}, {"op": "cbrt"}, {"op": "log"}, {"op": "exp"}
  ],
  "primary_units": {
    "Activation_Energy (eV)": "electron_volt",
    "Lattice_Constant_A (\AA)": "angstrom"
  },

  // ==================================================================
  //                     3. SEARCH & SELECTION STRATEGY
  // ==================================================================
  "max_D":                     3,
  "sis_sizes":                 [100],
  "search_strategy":           "rmhc",
  "max_feat_cross_correlation": 0.95,

  // ==================================================================
  //                   4. MODEL CONSTRUCTION & VALIDATION
  // ==================================================================
  "task_type":                 "regression",
  "selection_method":          "cv",
  "cv":                        10,
  "fix_intercept":             false,

  // ==================================================================
  //                         5. COMPUTATIONAL SETTINGS
  // ==================================================================
  "n_jobs":                    -1,
  "device":                    "cpu",
  "random_state":              42
}
```

Listing 1: An example configuration file for a materials science regression task.

# B Usage of run_discover.py

The primary entry point for running a DISCOVER analysis is the command-line script run_discover.py. It orchestrates the entire workflow, from data loading to model fitting and results serialization.

## Execution

To execute a run, a user needs two files:

1. A data file in CSV format.
2. A configuration file in JSON format (as described in Section A).

The script is invoked from the terminal, passing the path to the configuration file as the sole argument:

```
$ python run_discover.py path/to/your/config.json
```

## Workflow

Upon execution, the script performs the following steps:

1. **Load Configuration**: Parses the specified JSON file.
2. **Prepare Workspace**: Creates the output directory specified by workdir. It includes a safety prompt to prevent accidental overwriting of existing results.
3. **Load Data**: Reads the CSV file specified by data_file using pandas. It separates the target property (property_key) from the primary features and handles missing values by dropping the corresponding rows.
4. **Initialize Model**: Selects the appropriate model class (e.g., DiscoverRegressor, DiscoverClassifier) based on the task_type in the configuration.
5. **Run DISCOVER**: The .fit(X, y) method is called. This is the main computational step, which involves:
    - Iterative feature generation and screening up to the specified depth.
    - Search for the best D-dimensional models using the chosen search_strategy.
    - Model selection via the specified selection_method (e.g., CV) to determine the optimal dimension D.
    - Final model fitting and diagnostic calculations (VIF, coefficient errors).
6. **Save Results**: The script saves a comprehensive set of results to the workdir:
    - SISSO.out: A human-readable summary report of the final model, including its formula, performance metrics, and diagnostics.
    - final_models_summary.json: A structured JSON file containing detailed information for each dimensional model found, including features, coefficients, and scores. This is ideal for programmatic post-processing and plotting.
    - top_sis_candidates.csv: A CSV file ranking the top individual features from the final screened space by their correlation with the target, along with their single-feature $R^2$ and RMSE.
    - symbol_map.json: A JSON file mapping the internal symbolic names (f0, f1, ...) back to the original feature names from the input data file.
    - plots/: A directory containing plots for model selection (selection_scores.png), parity, etc.
    - models/: A directory containing detailed .dat files for each dimensional model, including its formula and coefficients.
7. **Print Summary**: The final model report is printed to the console.

### Illustrative Code Snippet

The core logic of `run_discover.py` demonstrates its role as a high-level driver.

```python
# ... (imports and argument parsing) ...
import json
import pandas as pd
from pathlib import Path
from discover import DiscoverRegressor, DiscoverClassifier

def run_analysis(config_path):
    # 1. Load Configuration
    with open(config_path, 'r') as f:
        # Note: Added logic to handle comments in the JSON file
        lines = [line for line in f if not line.strip().startswith('//')]
        config = json.loads("".join(lines))

    # 2. Prepare Directories and Data
    workdir = Path(config.get('workdir', 'discover_output'))
    # ... (directory setup logic) ...
    data = pd.read_csv(config.get('data_file'))
    y = data[config.get('property_key')]
    feature_cols = [c for c in data.columns if c not in [config.get('property_key')] +
    config.get('non_feature_cols', [])]
    X = data[feature_cols]

    # 3. Initialize and Run the Correct DISCOVER Model
    task_map = {
        'regression': DiscoverRegressor,
        'classification_svm': DiscoverClassifier,
        # ... other task types
    }
    task_key = config.get('task_type', 'regression').lower()
    DiscoverClass = task_map.get(task_key)

    print("\n--- Initializing and running DISCOVER ---")
    discover = DiscoverClass(**config)
    discover.fit(X, y)

    # 4. Save Additional Results and Print Final Report
    print("\n--- Saving additional results for plotting ---")
    # ... (logic to save top_sis_candidates.csv, final_models_summary.json)

    print("\n--- FINAL MODEL REPORT ---")
    print(discover.summary_report(X, y, sample_weight=None))
```

Listing 2: Core logic of the `run_discover.py` script.
